# Supplementary material for: Nonlinear Model Reduction to Temporally Aperiodic Spectral Submanifolds
Source: arXiv:2404.05355 source file (2024-04-08)
Supplement: Supplementary file 1 [file Existence_and_Computation_of_Hyperbolic_Trajectori.pdf]

ResearchGate

See discussions, stats, and author profiles for this publication at: https://www.researchgate.net/publication/220264964

# Existence and Computation of Hyperbolic Trajectories of Aperiodically Time Dependent Vector Fields and Their Approximations

**Article** *in* International Journal of Bifurcation and Chaos · June 2003

DOI: 10.1142/S0218127403007321 · Source: DBLP

CITATIONS
41

READS
137

**3 authors**, including:

Ning Ju
Oklahoma State University - Stillwater
**30** PUBLICATIONS **1,113** CITATIONS

SEE PROFILE

Stephen Wiggins
University of Bristol
**454** PUBLICATIONS **23,052** CITATIONS

SEE PROFILE

All content following this page was uploaded by Stephen Wiggins on 05 June 2014.

The user has requested enhancement of the downloaded file.

Papers

International Journal of Bifurcation and Chaos, Vol. 13, No. 6 (2003) 1449–1457
© World Scientific Publishing Company

# EXISTENCE AND COMPUTATION OF HYPERBOLIC TRAJECTORIES OF APERIODICALLY TIME DEPENDENT VECTOR FIELDS AND THEIR APPROXIMATIONS

NING JU
*Department of Mathematics, Duke University, Durham, NC 27708-0320, USA*

DES SMALL and STEPHEN WIGGINS*
*School of Mathematics, University of Bristol, University Walk, Bristol, BS8 1TW, UK*

Received April 12, 2002; Revised April 29, 2002

In this paper we give sufficient conditions for the existence of hyperbolic trajectories in aperiodically time dependent vector fields. These conditions do not require the *a priori* introduction of hyperbolicity into the dynamics of the vector field or assumptions of "time scale separation". The hyperbolic trajectory is obtained as a solution of an integral equation over an infinite time interval. We give an expression for the error obtained when the solution is approximated over a finite time interval. Finally, we show how the method can be numerically implemented in a specific example.

*Keywords*: Aperiodically time dependent vector field; hyperbolic trajectory; exponential dichotomy.

## 1. Introduction

Hyperbolicity is an important property of trajectories and invariant sets in dynamical systems. In the mathematical development of the subject, some hyperbolic properties are typically assumed, and the consequences are investigated. However, from the point of view of applications, it is important to have techniques that allow one to determine the existence of hyperbolic trajectories and invariant sets in specific dynamical systems.

For discrete time systems (maps) Newton's method is an efficient technique for finding periodic orbits, whose hyperbolicity properties can also be checked numerically. This method can be applied to time-periodic vector fields as well by considering the associated Poincaré map. However, for nonautonomous vector fields that are aperiodic in time (i.e. not periodic), we know of no generally applicable methods for finding hyperbolic trajectories. This is the subject of this paper.

Our approach bears some similarities to "integral manifold theorems" (see, e.g. [Henry, 1981; Yi, 1993; Sakamoto, 1994], and the references contained in these works for the history of integral manifolds). However, from the point of view of applications, there is a very important difference. The set-up for all of these theorems assumes an underlying unperturbed problem that contains a (normally) hyperbolic invariant manifold. The substance of these theorems then involves showing that these invariant manifolds persist, with similar properties, when more complicated "higher order" terms are included. In applications, it is generally not possible to separate a vector field into an unperturbed and perturbed part, where the unperturbed part contains a hyperbolic trajectory, or normally

*This research was supported by ONR Grant No. N00014-01-1-0769.

hyperbolic invariant manifold. Moreover, this approach involves the introduction of hyperbolicity into the initial set-up of the problem (i.e. hyperbolicity in the unperturbed problem). It is not clear how to do this in general applications. One would like techniques to determine the existence of hyperbolicity in given systems, without assuming some aspect of the property, *a priori*. Our work provides one way of doing this.

In this paper we feel that we have taken some steps in solving this problem in a specific setting which is applicable to problems related to transport and stirring in fluid flows. In the last ten years or so, much enthusiasm has arisen for the application of the dynamical systems approach to the study of problems concerned with mixing and transport in fluid mechanics; see for example [Ottino, 1989; Wiggins, 1992]. The analogy between the global dynamical, geometrical behaviors of nonlinear dynamical systems and Lagrangian transport and mixing in fluid flows has been manipulated to obtain a deeper understanding of Lagrangian transport issues in a variety of fluid flows. New results from experimental and numerical simulations and theoretical studies have been obtained for special classes of flows, which include time-periodic flows, quasiperiodic flows, adiabatic flows, and almost periodic flows. For examples, see the references cited in [Haller & Poje, 1998; Malhotra & Wiggins, 1998].

In these applications it is natural to freeze the time variable in the nonautonomous vector field and examine the equilibrium points of the frozen time vector field. One can also examine how these "move" in time by examining them at different times (in this way, the "time" in the expression for the vector field plays the role of a parameter). The reason this is natural in the fluid mechanical setting is that it corresponds to the Eulerian view of fluid mechanics. In many flow visualization settings one takes a "snapshot" of the velocity field at a fixed time and tries to determine certain features or structures in the resulting picture. "Frozen time stagnation points" are a typical structure fluid mechanicians focus on.

Of course, these frozen time equilibria are not trajectories of the vector field. However, in situations where the time variation of the velocity field is "slow", then frozen time equilibria may stay close to a true trajectory of the vector field. This is intuitively clear from perturbation theory and, therefore, it is not surprising that such results have been used in many fields, often with no knowledge of the previous history. For example, applications of such results can be found in control theory see [Desoer, 1969], and the recent paper [Peuteman *et al.*, 2000] which contains historical references for control applications. In the context of fluid mechanics (Stokes flows) such results were used in [Kaper & Wiggins, 1993]. Recently, these results were further extended in [Haller & Poje, 1998]. In the purely mathematical context related results can be found in [Coppel, 1978, pp. 50 and 54].

However, in most fluid mechanical applications the velocity field is not slowly varying (in an appropriate sense) and the above results do not apply. In this paper we provide an existence criteria for hyperbolic trajectories that do not require restrictions on the rate of time variation of the vector field. However, we will still use frozen time hyperbolic equilibria as a feature of the vector field on which to focus our search for hyperbolic trajectories. This is not the same as introducing hyperbolicity into the *dynamics* of the vector field since these frozen time equilibria are not trajectories. Moreover, we will see that the curves of frozen time equilibria need not remain close to the hyperbolic trajectories that they give rise to.

This paper is organized as follows. In Sec. 2 we describe the set-up, define hyperbolicity of trajectories of nonautonomous vector fields in terms of exponential dichotomies, and give our main assumption on the existence of a curve of hyperbolic, "frozen time" equilibrium points for the vector field. In Sec. 2.1 we transform the original general vector field to a frame "moving" with the frozen time equilibrium points. We then give an integral equation and a theorem stating that under certain conditions the integral equation has a unique, hyperbolic trajectory. In Sec. 3 we address the issue of approximation of hyperbolic trajectories over finite time intervals and give a theorem with convergence and error estimates. In Sec. 4 we describe a numerical approach for solving for the hyperbolic trajectories and carry out its implementation for a specific example. In order to make the presentation proceed more smoothly we present no proofs of results in the main body of the text. This is compared with a related linear algorithm given in [Ide *et al.*, 2002] and our results can be viewed as a rigorous extension of this algorithm to the nonlinear setting. The proofs are relegated to an appendix.

## 2. Existence and Equations for Hyperbolic Trajectories

We consider a general nonautonomous vector field:

$$\dot{y}(t) = v(y(t), t), \quad y \in R^n, \quad t \in R. \tag{1}$$

Our goal is to develop a technique for finding hyperbolic trajectories of (1). First we define this notion.

Hyperbolicity of a trajectory of (1) is a property of the linearized dynamics about the trajectory. To quantify this, we need a preliminary definition.

**Definition 2.1** (Exponential Dichotomy). Let $X(t)$ be the fundamental solution matrix of the linear equation:

$$\dot{x} = A(t)x. \tag{2}$$

where $A(t)$ is an $n \times n$ matrix, continuous for $t \in R$. Equation (2) is said to have an *exponential dichotomy* if there exists a projection $P$, i.e. a matrix $P$, such that $P^2 = P$, and positive constants $K$, $L$, $\alpha$ and $\beta$ such that:

$$\begin{aligned} |X(t)PX^{-1}(s)| &\le Ke^{-\alpha(t-s)}, \quad s \le t < \infty, \\ |X(t)QX^{-1}(s)| &\le Le^{-\beta(s-t)}, \quad s \ge t > -\infty. \end{aligned} \tag{3}$$

where $Q = I - P$ and $I$ is the identity matrix.

There is a large literature on exponential dichotomies. See, for example [Massera & Schäffer, 1966; Coppel, 1978] or [Henry, 1981].

With the definition of exponential dichotomy in hand, we can now define what it means for a trajectory of (1) to be hyperbolic.

**Definition 2.2** (Hyperbolic Trajectory). A trajectory $y_h(t)$ of (1) is said to be *hyperbolic* if the linearized equation:

$$\dot{\xi} = \frac{\partial v}{\partial y}(y_h(t), t)\xi, \quad \xi \in R^n.$$

has an exponential dichotomy.

We next introduce the assumption on (1) that will provide the basis for our search for hyperbolic trajectories.

**Assumption 2.1** (Curve of Hyperbolic Instantaneous Equilibrium Points). We assume that there exists a $C^1$ curve of instantaneous equilibrium points $y_e(t)$, $t \in R$, for (1), i.e.

$$v(y_e(t), t) = 0, \quad t \in R. \tag{4}$$

We further assume that the curve of instantaneous equilibrium points is hyperbolic in the sense that the linear equation:

$$\dot{\xi} = \frac{\partial v}{\partial y}(y_e(t), t)\xi, \quad \xi \in R^n. \tag{5}$$

has an exponential dichotomy.

It is a simple matter to verify that $y_e(t)$ is not a trajectory of (1) unless $\dot{y}_e(t) = 0$. This is an important point to realize as the notion of hyperbolicity is typically applied to trajectories or invariant sets. Here we will be defining hyperbolicity of a set that is neither.

### 2.1. *Localization about the instantaneous equilibrium points*

Next we transform (1) to a frame moving with the instantaneous equilibrium points. It is easy to see that

$$\begin{aligned} \frac{d}{dt}(y(t) - y_e(t)) &= \nabla v(y_e(t), t)(y(t) - y_e(t)) \\ &\quad + [v(y, t) - \nabla v(y_e(t), t)(y(t) \\ &\quad - y_e(t)) - \dot{y}_e(t)], \end{aligned} \tag{6}$$

where $y \in R^n$, $t \in R$ and $\nabla v(y_e(t), t) := (\partial v/\partial y)(y, t)|_{y=y_e(t)}$.

We define:

$$x(t) := y(t) - y_e(t), \tag{7}$$

$$A(t) := \nabla v(y_e(t), t), \tag{8}$$

$$\begin{aligned} f(x, t) &:= v(y, t) - \nabla v(y_e(t), t)(y(t) \\ &\quad - y_e(t)) - \dot{y}_e(t), \\ &= v(x + y_e(t), t) \\ &\quad - \nabla v(y_e(t), t)x(t) - \dot{y}_e(t). \end{aligned} \tag{9}$$

Then (1) takes the general form:

$$\dot{x}(t) = A(t)x(t) + f(x(t), t), \qquad x \in R^n, \quad t \in R, \tag{10}$$

Associated to (10) we have the following integral equation:

$$\begin{aligned} x(t) &= X(t)\int_{-\infty}^{t} PX^{-1}(s)f(x(s), s)ds \\ &\quad - X(t)\int_{t}^{\infty} QX^{-1}(s)f(x(s), s)ds, \end{aligned} \tag{11}$$

where $P$ and $Q$ are the projections associated with the exponential dichotomy of (5) and $X(t)$ is the fundamental solution matrix of (5). It is a straightforward calculation to show that a solution of (11) is a solution of (10).

Now, if we can find a hyperbolic trajectory of (10), $x_h(t)$, then $y_h(t) := x_h(t) + y_e(t)$ is a hyperbolic trajectory of (1).

## 2.2. *Existence, uniqueness and hyperbolicity*

Now we prove a theorem which provides conditions for (11) to have a unique solution which is a hyperbolic trajectory of (10).

**Theorem 2.1.** *Suppose Assumption 2.1 holds. Suppose further that*

$$\|v(y(\cdot), \cdot) - \nabla v(y_e(\cdot), \cdot)(y(\cdot) - y_e(\cdot)) - \dot{y}_e(\cdot)\|_\infty < \infty\,, \tag{12}$$

*and*

$$\|\nabla v(y(\cdot), \cdot) - \nabla v(y_e(\cdot), \cdot)\|_\infty < \left(\frac{K}{\alpha} + \frac{L}{\beta}\right)^{-1}. \tag{13}$$

*Then, there exists a unique hyperbolic trajectory $y_h(t) = x_h(t) + y_e(t)$ for (1), where $x_h(t)$ is the unique solution of the nonlinear integral equation (11).*

The proof is given in the appendix.

- The integral equation (11) is similar to the type of integral equation arising in the study of integral manifolds (see, e.g. [Henry, 1981; Yi, 1993], or [Sakamoto, 1994]). The difference in our context lies on the derivation and assumptions on (10). In particular, we do not assume hyperbolicity *of trajectories* in the vector field, or in any part of it (i.e. an "unperturbed" part). Hyperbolicity arises from a "nondynamical" effect: hyperbolic instantaneous equilibrium points of the "frozen time" vector field.
- The bound in (13) is expressed entirely in terms of the constants in the exponential dichotomy definition. Numerical methods for calculating these constants are given in [Dieci *et al.*, 1997].

# 3. Approximation Over Finite Time Intervals

In most practical situations, (11) will have to be solved numerically. Practically speaking, this can only be carried out over a finite time interval. We now derive some estimates on the error incurred as a result.

Considering (11), it is natural to define the concept of *approximate* hyperbolic trajectory as follows.

**Definition 3.1.** We define the approximate hyperbolic trajectory on the interval $[T_1, T_2]$, denoted $x_a(t)$, as a solution of the following equation:

$$x_a(t) = X(t)\int_{T_1}^{t} PX^{-1}(s)f(x_a(s), s)ds - X(t)\int_{t}^{T_2} QX^{-1}(s)f(x_a(s), s)ds\,. \tag{14}$$

Then we have the following result.

**Theorem 3.1.** *Under the conditions of Theorem A.1 (which are relaxed such that they hold in the domain $[T_1, T_2]$ instead of $R$) there is a unique approximate hyperbolic trajectory defined on the interval $[T_1, T_2]$ in the sense of Definition 3.1.*

The proof of this theorem follows precisely the same line of argument as the proof of Theorem A.4.2, with certain obvious modifications for the finite time interval and is therefore omitted.

As a corollary, under the condition of Theorem A.4.2, when there is a unique hyperbolic trajectory, there is also a unique approximate hyperbolic trajectory in the sense of Definition 3.1 on every interval $[T_1, T_2]$.

Moreover, we have the following error estimate and convergence result.

**Theorem 3.2.** (*Error Estimate and Convergence*). *Under the conditions of Theorem A.4.2,*

$$\|x_a(t) - x_h(t)\|_{C[T_1,T_2]} \le \left[1 - \|f_x\|_\infty\left(\frac{K}{\alpha} + \frac{L}{\beta}\right)\right]^{-1} \times \left\{\max_{T_1\le t}\left|\int_{-\infty}^{T_1} X(t)PX^{-1}(s)f(x_h(s), s)ds\right| + \max_{t\le T_2}\left|\int_{T_2}^{\infty} X(t)QX^{-1}(s)f(x_h(s), s)ds\right|\right\}. \tag{15}$$

*Suppose further that*

$$\lim_{T_1\to-\infty}\max_{T_1\le t}\left|\int_{-\infty}^{T_1} X(t)PX^{-1}(s)f(x_h(s),\,s)ds\right| = 0\,, \tag{16}$$

*and that*

$$\lim_{T_2\to\infty}\max_{t\le T_2}\left|\int_{T_2}^{\infty} X(t)QX^{-1}(s)f(x_h(s),\,s)ds\right| = 0\,. \tag{17}$$

*Then*

$$\lim_{-T_1,T_2\to\infty}\|x_a(t)-x_h(t)\|_{C[T_1,T_2]} = 0\,. \tag{18}$$

## 4. Numerical Solution for Computing Hyperbolic Trajectories

The theory developed for the existence of hyperbolic trajectories can be cast in an algorithmic form and implemented numerically. We describe the steps in this procedure, and their implementation in a specific example.

***Step 1.*** Find a curve of instantaneous equilibrium points of (1).

This is straightforward. However, since, for each $t$, (4) is a nonlinear algebraic equation its solution will generally have to be carried out numerically. This is a well-studied problem and there are many procedures for doing this (e.g. Newton's method). Nevertheless, it serves to highlight the finite time aspect of the problem from the start as this numerical procedure can only be carried out on a finite interval of $t$, say $[T_1,\,T_2]$ (if we were dealing with time-periodic vector fields this would not be an issue since it would be sufficient to solve (4) over one period).

***Step 2.*** Localize (1) about the curve of instantaneous equilibrium points by transforming (1) to (10).

Once the curve of instantaneous equilibrium points is obtained, this step is straightforward.

***Step 3.*** Verify that the curve of instantaneous equilibrium points is hyperbolic.

***Step 4.*** Solve the integral equations for a hyperbolic trajectory.

These are the most difficult steps and they are carried out together.

In verifying that the curve of instantaneous equilibrium points is hyperbolic we must deal with the issues related to the solution of the homogeneous problem associated with (10), $\dot{x} = A(t)x$. In particular, we must solve for the fundamental solution matrix $X(t)$ and then verify that it satisfies the criteria of exponential dichotomy given in Definition 2. Here we describe the numerical approach for solving these problems that was given in [Ide *et al.*, 2002].

It is shown in [Ide *et al.*, 2002] that there exists a linear, time dependent transformation:

$$w = T(t)x\,, \tag{19}$$

under which (10) becomes:

$$\dot{w} = Dw + h(w,\,t)\,, \tag{20}$$

where

$$D = \frac{1}{T_2 - T_1}\,\Sigma(T_2,\,T_1),$$

$$h(w,\,t) = T(t)f(T^{-1}(t)w,\,t)\,. \tag{21}$$

In general, this transformation can only be carried out numerically. The computer code for the calculations we do can be obtained at http://lacms.maths.bris.ac.uk. The transformation $T(t)$, the definition of $D$, and its relation to the fundamental solution matrix $X(t)$ is given explicitly in the appendix, where it is shown that $D$ is a diagonal matrix, and its matrix elements are the finite time Lyapunov exponents of the fundamental solution matrix $X(t)$. Hence, $X(t)$ satisfies an exponential dichotomy if and only if $D$ has no eigenvalues with zero real parts.

We denote the matrix elements of $D$ by $d_{i,i} \equiv d_i$, and we suppose that $d_i < 0$, $1 \le i \le k$ and $d_i > 0$, $k+1 \le i \le n$. Then the analog of (11) in the $w$ coordinates is given by:

$$w_i(t) = \begin{cases} \displaystyle\int_{T_1}^{t} e^{d_i(t-s)}h_i(w(s),s)ds, & 1\le i\le k,\\[2ex] \displaystyle -\int_{t}^{T_2} e^{d_i(t-s)}h_i(w(s),s)ds, & k+1\le i\le n. \end{cases} \tag{22}$$

The numerical solution of Eq. (22) [and thus Eq. (10)] may be calculated using essentially the

same iterative procedure as is used in the proof of Theorem A.4.2 as follows:

(1) We take $w^0(t) = 0$ as an initial estimate.
(2) Given $w^i(t)$ we calculate $h^i(w, t) = h(w^i(t), t)$.
(3) The quadratures of Eq. (22) are then calculated using $h^i(w, t)$ to give $w^{i+1}(t)$.

This process is iterated until a fixed point $w^{n+1}(t) \simeq w^n(t)$ is achieved to a suitable tolerance. The solutions are then transformed back into the $x$ coordinates using the inverse of (19).

## 4.1. *Results*

The algorithm described above was tested with the two-dimensional rotating Duffing system,

$$\begin{pmatrix} \dot{y}_1 \\ \dot{y}_2 \end{pmatrix} = \begin{pmatrix} \sin 2\beta t & \beta + \cos 2\beta t \\ -\beta + \cos 2\beta t & -\sin 2\beta t \end{pmatrix} \begin{pmatrix} y_1 \\ y_2 \end{pmatrix} + [-(y_1 \cos \beta t - y_2 \sin \beta t)^3 + \varepsilon \sin \omega t] \begin{pmatrix} \sin \beta t \\ \cos \beta t \end{pmatrix}. \tag{23}$$

The particular case shown in Fig. 1 is that with $\omega = 1$, $\varepsilon = 0.1$, $\beta = 0.3$ with 100 time steps in 10 time units. Note that the vector field does not have period 10 for these parameter values. It is effectively a finite time, aperiodic vector field.

Figure 1 shows clearly that the path of the instantaneous equilibrium point, $y^0$ is not a good prediction of the hyperbolic trajectory, but that $y^1$ already is. Successive iterations in this case do not greatly change the predicted trajectory, and the algorithm in fact converges after 14 iterations.

## 4.2. *Comparison with the algorithm of* [*Ide et al., 2002*]

Ide *et al.* [2002] developed an algorithm to find hyperbolic trajectories for velocity fields defined as data sets that essentially boils down to solving a version of (10) where the inhomogeneous forcing term $f(x, t)$ is only a function of $t$, i.e. it is a linear system. Our work here generalizes that algorithm and provides convergence results.

In particular $f(x, t)$ may be written as

$$f(x, t) = f_1(x, t) + f_2(t) \tag{24}$$

where $f_1(x, t) = v(x + y_s(t), t) - Ax$ and $f_2(t) = -\dot{y}(t)$. The term $f_2(t)$ is included in the calculations of Ide *et al.* [2002], but the term $f_1(x, t)$ is not.

Note that the definition of $w^0$ implies that $f_1 = 0$ in this case, so that $w^1(t)$ gives the same estimate of the hyperbolic trajectory as in [Ide *et al.*, 2002].

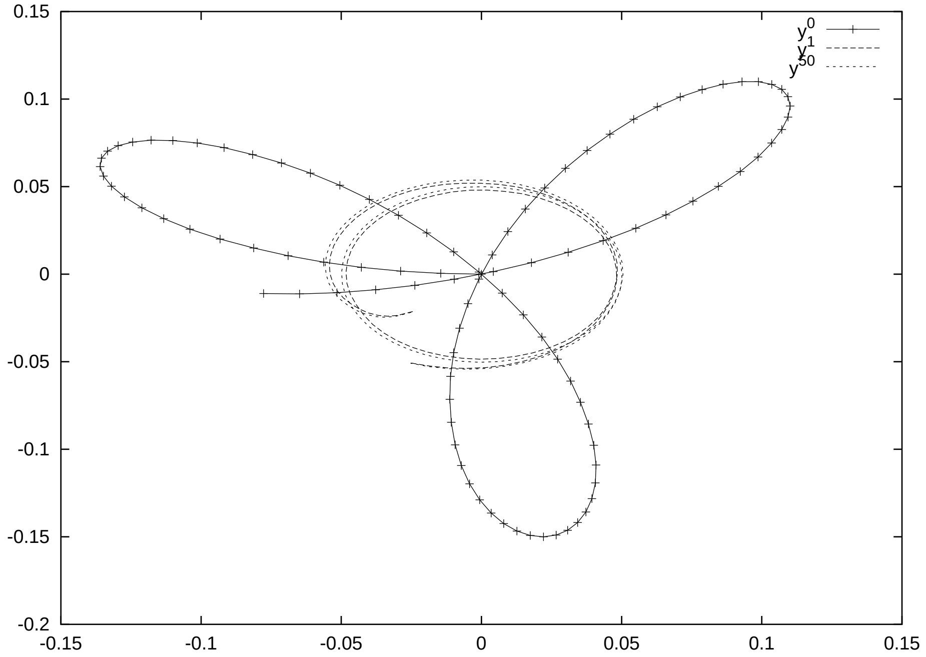


Fig. 1. Convergence of the algorithm. $y^0$ denotes the path of the instantaneous equilibrium point, which bears no geometrical relation to the hyperbolic trajectory.

## Acknowledgment

We are grateful to Kayo Ide for many illuminating discussions.

## References

Coppel, W. A. [1978] *Dichotomy in Stability Theory*, Lecture Notes in Mathematics, Vol. 629 (Springer-Verlag, NY, Heidelberg, Berlin).

Desoer, C. A. [1969] "Slowly varying $\dot{x} = A(t)x$," *IEEE Trans. Automat. Contr.* **14**, 1091–1100.

Dieci, L., Russell, R. D. & Van Vleck, E. S. [1997] "On the computation of Lyapunov exponents for continuous dynamical systems," *SIAM J. Numer. Anal.* **34**, 402–423.

Dieci, L. & Eirola, T. [1999] "On smooth decompositions of matrices," *SIAM J. Matrix Anal. Appl.* **20**, 800–819.

Haller, G. & Poje, A. [1998] "Finite time transport in aperiodic flows," *Physica* **D119**, 352–380.

Henry, D. [1998] *Geometric Theory of Semilinear Parabolic Equations*, Lecture Notes in Mathematics, Vol. 840 (Springer-Verlag, NY, Heidelberg, Berlin).

Ide, K., Small, D. & Wiggins, S. [2002] "Distinguished hyperbolic trajectories in time dependent fluid flows: Analytical and computational approach for velocity fields defined as data sets," *Nonlin. Process. Geophys.* **9**, 237–263.

Ju, N. & Wiggins, S. [2001] "On roughness of exponential dichotomy," *J. Math. Anal. Appl.* **262**, 39–49.

Kaper, T. J. & Wiggins, S. [1993] "An Analytical study of transport in stokes flows exhibiting large scale chaos — The eccentric journal bearing," *J. Fluid Mech.* **253**, 211–243.

Malhotra, N. & Wiggins, S. [1998] "Geometric structures, lobe dynamics, and Lagrangian transport in flows with aperiodic time-dependence, with applications to Rossby wave flow," *J. Nonlin Sci.* **8**, 401–456.

Massera, J. L. & Schäffer, J. J. [1996] *Linear Differential Equations and Function Spaces* (Academic Press, NY).

Ottino, J. [1989] *The Kinematics of Mixing: Stretching, Chaos, and Transport* (Cambridge University Press, Cambridge).

Peuteman, J., Aeyels, D. & Sepulchre, R. [2000] "Boundedness properties for time-varying nonlinear systems," *SIAM J. Contr. Optim.* **39**, 1408–1422.

Sakamoto, K. [1994] "Estimates on the strength of exponential dichotomies and application to integral manifolds," *J. Diff. Eqs.* **107**, 259–279.

Wiggins, S. [1992] *Chaotic Transport in Dynamical Systems* (Springer, NY).

Yi, Y. [1993] "A generalized integral manifold theorem," *J. Diff. Eqs.* **102**, 153–187.

## Appendix A
## Proofs of the Theorems

### A.1. *Proof of Theorem 2.1*

First we prove existence and uniqueness of solutions to the integral equation (11). Afterwards, we prove that the solution obtained in this way is hyperbolic.

**Theorem A.1** (Uniqueness and Existence). *Suppose that in (10) $\|f\|_\infty$, $\|f_x\|_\infty < \infty$ and that*

$$\|f_x\|_\infty \left(\frac{K}{\alpha} + \frac{L}{\beta}\right) < 1\,. \tag{A.1}$$

*Then (11) has a unique* bounded *and* continuous *solution that is a trajectory of (10), denoted $x_h(t)$.*

*Proof.* Let $BC[R^1; R^n]$ denote the space of all bounded and continuous functions defined on $R^1$ with values in $R^n$. It is easy to see that $BC[R^1; R^n]$ is a Banach space. Now define a map $\mathcal{T}$ from $BC[R^1; R^n]$ to itself as follows.

$$\begin{aligned}\mathcal{T}x(t) = X(t)\int_{-\infty}^{t} PX^{-1}(s)f(x(s), s)ds \\ - X(t)\int_{t}^{\infty} QX^{-1}(s)f(x(s), s)ds\,.\end{aligned} \tag{A.2}$$

Then, using the exponential dichotomy, it is easy to see that $\mathcal{T}x(t)$ defines a bounded differentiable function for any continuous function $x(t)$. That is $\mathcal{T}$ is well defined in $BC[R^1; R^n]$.

Notice that

$$\begin{aligned}\mathcal{T}x_1(t) - \mathcal{T}x_2(t) = X(t)\int_{-\infty}^{t} PX^{-1}(s)[f(x_1(s), s) \\ - f(x_2(s), s)]ds\,, \\ - X(t)\int_{t}^{\infty} QX^{-1}(s)[f(x_1(s), s) \\ - f(x_2(s), s)]ds\end{aligned} \tag{A.3}$$

Then the theorem follows from the use of the exponential dichotomy again and the contraction mapping principle. ∎

Now in order to check the hyperbolicity of the trajectories we found in the above theorems we need to check that the vector field linearized about the trajectory has an exponential dichotomy. The appropriate linearized vector field is given by:

$$\dot{z}(t) = (A(t) + D_x f(x_h(t), t))z(t)\,. \tag{A.4}$$

First we recall the following recent perturbation theorem for exponential dichotomies given in [Ju & Wiggins, 2001]:

**Theorem A.2** [Ju & Wiggins, 2001]. *Suppose* $\dot{x} = A(t)x$ *has an exponential dichotomy on* $R$ *with positive constants* $K_1$, $K_2$, $\alpha_1$, $\alpha_2$, *and projection* $P$. *Suppose further*

$$\sup_{t\in R} |B(s)| \left\{ \frac{K_1}{\alpha_1} + \frac{K_2}{\alpha_2} \right\} < 1\,, \tag{A.5}$$

*Then*

$$\dot{y}(t) = [A(t) + B(t)]y(t) \tag{A.6}$$

*also has an exponential dichotomy on* $R$ *with* $K_1 = K_2 = K > 0$, $\alpha_1 = \alpha_2 = \alpha > 0$, *and projection* $P'$. *Moreover, the projection* $P'$ *is similar to* $P$ *and one has that*

$$\|Y(t)P'Y^{-1}(t) - X(t)PX^{-1}(t)\| \le 2K^2 \quad \forall\, t \in R\,. \tag{A.7}$$

*where* $Y(t)$ *denotes the fundamental solution matrix of (A.6).*

Notice that under the conditions given in Theorem A.4.2, the conditions of Theorem A.2 are satisfied. Thus we immediately have the following important result.

**Theorem A.3** (Hyperbolicity). *Under the condition (A.1) the unique solution* $x_h(t)$ *as the fixed point of* $\mathcal{T}$, *defined by (A.2), is hyperbolic in the sense that the exponential dichotomy property holds for* $x_h(t)$.

The roughness theorem for exponential dichotomies given in [Ju & Wiggins, 2001] is an improvement over previous results in that the matrix $A(t)$ can become unbounded as $t \to \pm\infty$. Recalling the definition of $A(t)$ given in (8), this means that the curve of instantaneous equilibrium points, $y_e(t)$, can become unbounded as $t \to \pm\infty$. This behavior may occur in the applications to fluid transport that we have described in the introduction.

## A.2. *Proof of Theorem 3.2*

By (11) and (14), we have

$$\begin{aligned} x_h(t) - x_a(t) = X(t) &\int_{-\infty}^{T_1} PX^{-1}(s) f(x_h(s), s)ds \\ &+ X(t)\int_{T_1}^{t} PX^{-1}(s)[f(x_h(s), s) \\ &- f(x_a(s), s)]ds \\ &- X(t)\int_{t}^{T_2} QX^{-1}(s)[f(x_h(s), s) \\ &- f(x_a(s), s)]ds \\ &- X(t)\int_{T_2}^{\infty} QX^{-1}(s) f(x_h(s), s)ds\,. \end{aligned}$$

Thus,

$$\begin{aligned} &\|x_a(t) - x_h(t)\|_{C[T_1,T_2]} \\ &\quad\le \max_{t\in[T_1,T_2]} \left| \int_{-\infty}^{T_1} X(t)PX^{-1}(s)f(x_h(s),s)ds \right| \\ &\qquad + \left| \int_{T_1}^{t} X(t)PX^{-1}(s)[f(x_h(s),s) - f(x_a(s),s)]ds \right| \\ &\qquad + \left| \int_{t}^{T_2} X(t)QX^{-1}(s)[f(x_h(s),s) - f(x_a(s),s)]ds \right| \\ &\qquad + \max_{t\in[T_1,T_2]} \left| \int_{T_2}^{\infty} X(t)QX^{-1}(s)f(x_h(s),s)ds \right| \end{aligned} \tag{A.8}$$

Using (3) gives:

$$\begin{aligned} &\|x_a(t) - x_h(t)\|_{C[T_1,T_2]} \\ &\quad\le \max_{T_1\le t} \left| \int_{-\infty}^{T_1} X(t)PX^{-1}(s)f(x_h(s),s)ds \right| \\ &\qquad + \|f_x\|_\infty \left( \frac{K}{\alpha} + \frac{L}{\beta} \right) \|x_a(t) - x_h(t)\|_{C[T_1,T_2]} \\ &\qquad + \max_{t\le T_2} \left| \int_{T_2}^{\infty} X(t)QX^{-1}(s)f(x_h(s),s)ds \right| \end{aligned}$$

After rearranging terms and using (A.1), (15) follows.

Then (18) follows from (15) by using (16) and (17).

## A.3. *The transformation of the linear part of (10) to constant coefficient*

On the time interval $[T_1, T_2]$ let $X(t, T_1)$ denote the fundamental solution matrix of $\dot{x} = A(t)x$, with $X(T_1, T_1) = I$. First we need to describe how to solve for the fundamental solution matrix. In the hyperbolic situation, standard "of the shelf" integrators often lead to solutions that blow up exponentially and rapidly exceed machine precision.

There has been much work on this in recent years. A numerically stable approach is to write the fundamental solution matrix in the form of a QR or singular value decomposition (see, e.g. [Dieci *et al.*, 1997; Dieci & Eirola, 1999] or [Ide *et al.*, 2002]). We follow the latter approach and represent the fundamental solution matrix in the form of a singular value decomposition:

$$X(t, T_1) = B(t, T_1) \exp(\Sigma(t, T_1)) R(t, T_1)^T \,,$$

where $B(t, T_1)$ and $R(t, T_1)$ are orthogonal matrices, i.e. $B(t, T_1)B(t, T_1)^T = R(t, T_1)R(t, T_1)^T = I$, and $\Sigma(t, T_1)$ is a diagonal matrix with $\Sigma(T_1, T_1) = 0$ so that $\exp(\Sigma(t, T_1))$ is a diagonal matrix with $\exp(\Sigma(T_1, T_1)) = I$. It is shown in [Ide *et al.*, 2002] that there exists a time-dependent, linear transformation:

$$w = T(t)x \,,$$

where

$$T(t) = \exp((t - T_1)D)R(T_2, T_1)^T R(t, T_1) \times \exp(-\Sigma(t, T_1))B(t, T_1)^T \,,$$

which transforms (11) into (20), where

$$D = \frac{1}{T_2 - T_1} \Sigma(T_2, T_1) \,.$$

Thus, if $B(t, T_1)$, $\Sigma(t, T_1)$, and $R(t, T_1)$ are computed over the time interval $t \in [T_1, T_2]$ then the transformation to (22) can also be carried out.

A numerical procedure for calculating the matrices $B(t, T_1)$, $\Sigma(t, T_1)$, and $R(t, T_1)$ is given in [Ide *et al.*, 2002].
